# Supplementary material for: NeuralQA: A Usable Library for Question Answering (Contextual Query Expansion + BERT) on Large Datasets
Source: arXiv:2007.15211 source file (2020-11-28)
Supplement: Supplementary file 1 [file appendix.tex]

\newpage
\appendix

\section{Contextual Query Expansion: User in the Loop Workflow}
\label{sec:uiinteraction}
In this work we introduce contextual query expansion using masked language models. In this section, we discuss some insights on limitations of this approach and potential strategies to address them. First the underlying MLM model should be finetuned on the target corpus. Second, to reduce the possibility of introducing expansion terms that alter the semantic meaning of the overall query, conservative expansion rules are required that govern which candidate gets expanded.   Given these limitations, it makes sense that a user in the loop approach to query expansion where possible is useful. In this setup, the user provides

To aid in  reproducibility and benchmarking, CQE is  bundled as an independent section of the NeuralQA library. 

\paragraph{\LaTeX-specific details:}
Use {\small\verb|\appendix|} before any appendix section to switch the section numbering over to letters.

\section{Library Configuration}
\label{sec:configuration}
NeuralQA provides an yaml file based interface for specifying configurations for the library. In this section we outline a list of supported configuration parameters.

\section{Configuration}
\label{sec:configuration}
Nonetheless, supplementary material should be supplementary (rather than central) to the paper.
\textbf{Submissions that misuse the supplementary material may be rejected without review.}
Supplementary material may include explanations or details of proofs or derivations that do not fit into the paper, lists of
features or feature templates, sample inputs and outputs for a system, pseudo-code or source code, and data.
(Source code and data should be separate uploads, rather than part of the paper).

The paper should not rely on the supplementary material: while the paper may refer to and cite the supplementary material and the supplementary material will be available to the reviewers, they will not be asked to review the supplementary material.
